# Supplementary material for: Fabricating a dielectrophoretic microfluidic device using 3D-printed moulds and silver conductive paint
Source: arXiv:2302.10690 source file (2023-02-21)
Supplement: Supplementary file 1 [file Supporting_information.pdf]

# Fabricating a dielectrophoretic microfluidic device using 3D printed molds and silver conductive paint

Shayan Valijam[1,2], Dmitry Malyshev[2], Daniel P.G. Nilsson[2], Rasmus Öberg[2], and Magnus Andersson[2,3,*]

[1]Faculty of Electrical Engineering, K. N. Toosi University of Technology, Tehran, 1631714191, Iran

[2]Department of Physics, Umeå University, Umeå, 901 87, Sweden

[3]Umeå Center for Microbial Research (UCMR), Umeå, 901 87, Sweden

[*]Corresponding author: magnus.andersson@umu.se

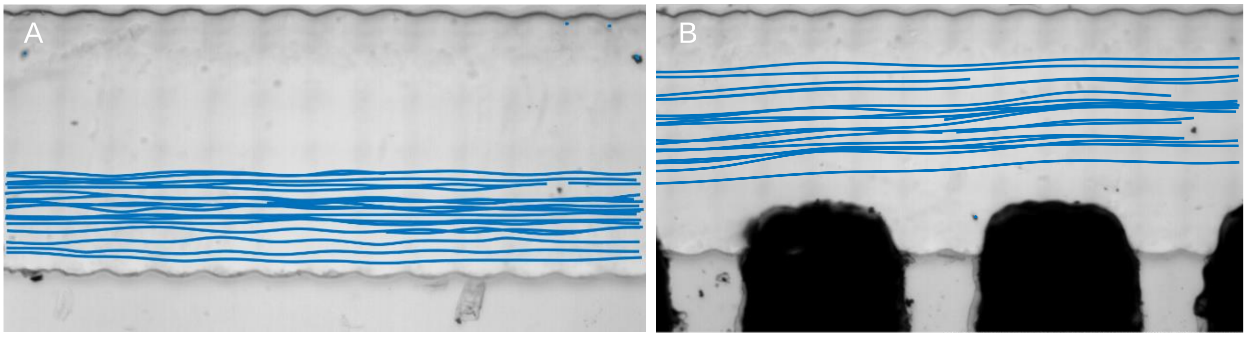


Figure S1. Examples of 10 µm particle trajectories A) before the electrodes and B) at the electrodes.

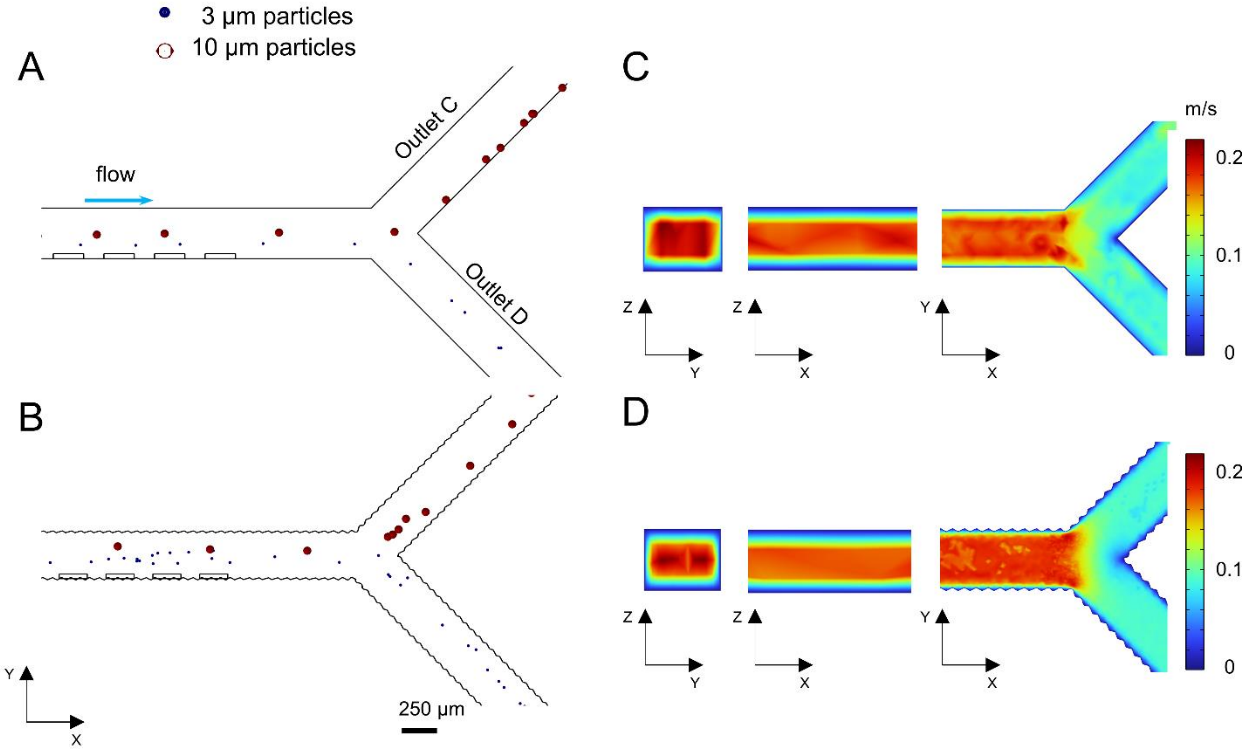


Figure S2. Still image from the simulation of the separation of particles with V ±11 V at 75 kHz. The wave like pattern does not interfere in the ability to separate the particles (A-B). The flow velocities inside the channel (C-D) are also similar.
